# Supplementary material for: First principles phase diagram calculation and theoretical investigation of electronic structure properties of $\mathrm{KCuTe_{1-x}Se_{x}}$ for photocathode applications
Source: arXiv:2501.02319 ancillary file (2025-01-04)
Supplement: Supplementary file 1 [file arini_SI.pdf]

**First principles phase diagram calculation and  
theoretical investigation of electronic structure  
properties of  $\text{KCuTe}_{1-x}\text{Se}_x$  for photocathode  
applications**

Arini Kar<sup>1</sup>, K. R. Balasubramaniam<sup>1</sup>, Dayadeep S. Monder<sup>1\*</sup>

<sup>1</sup>Department of Energy Science and Engineering, Indian Institute of Technology Bombay, Mumbai,  
Maharashtra 400076

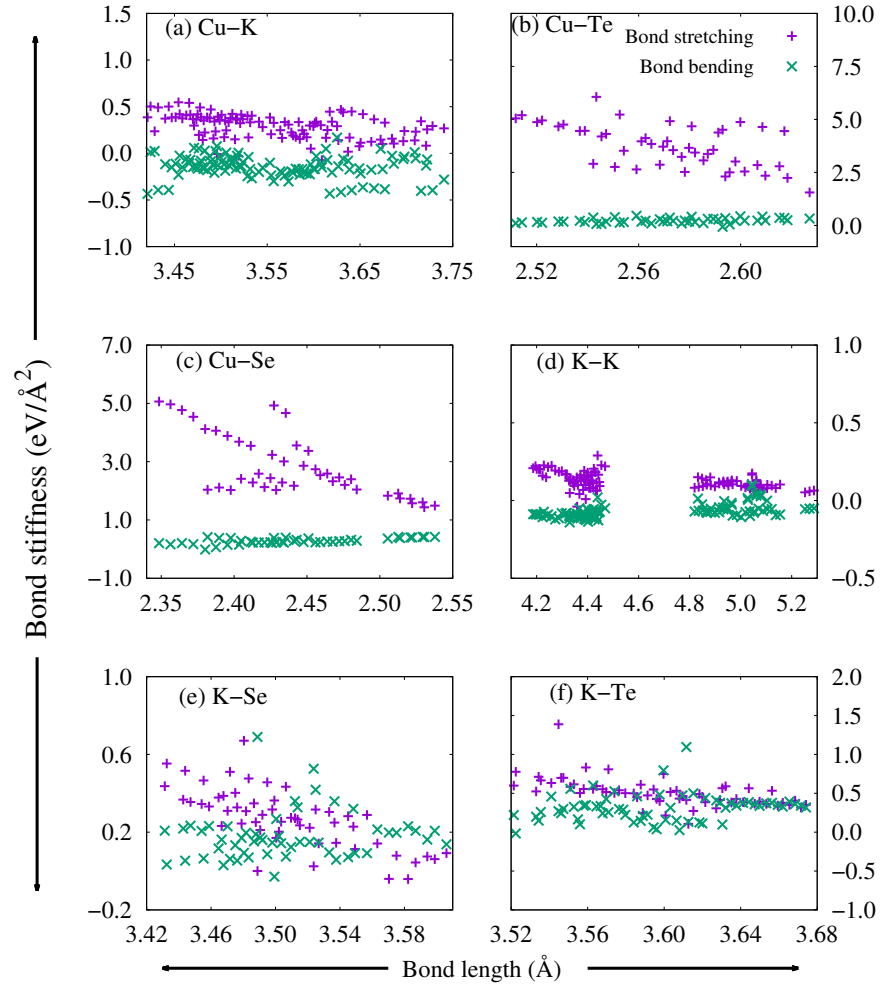

Figure S1: Plot of the bond length dependent transferable force constants of a) Cu-K b) Cu-Te c) Cu-Se d) K-K e) K-Se f) K-Te bonds in  $\text{KCuTe}_{1-x}\text{Se}_x$  alloy.

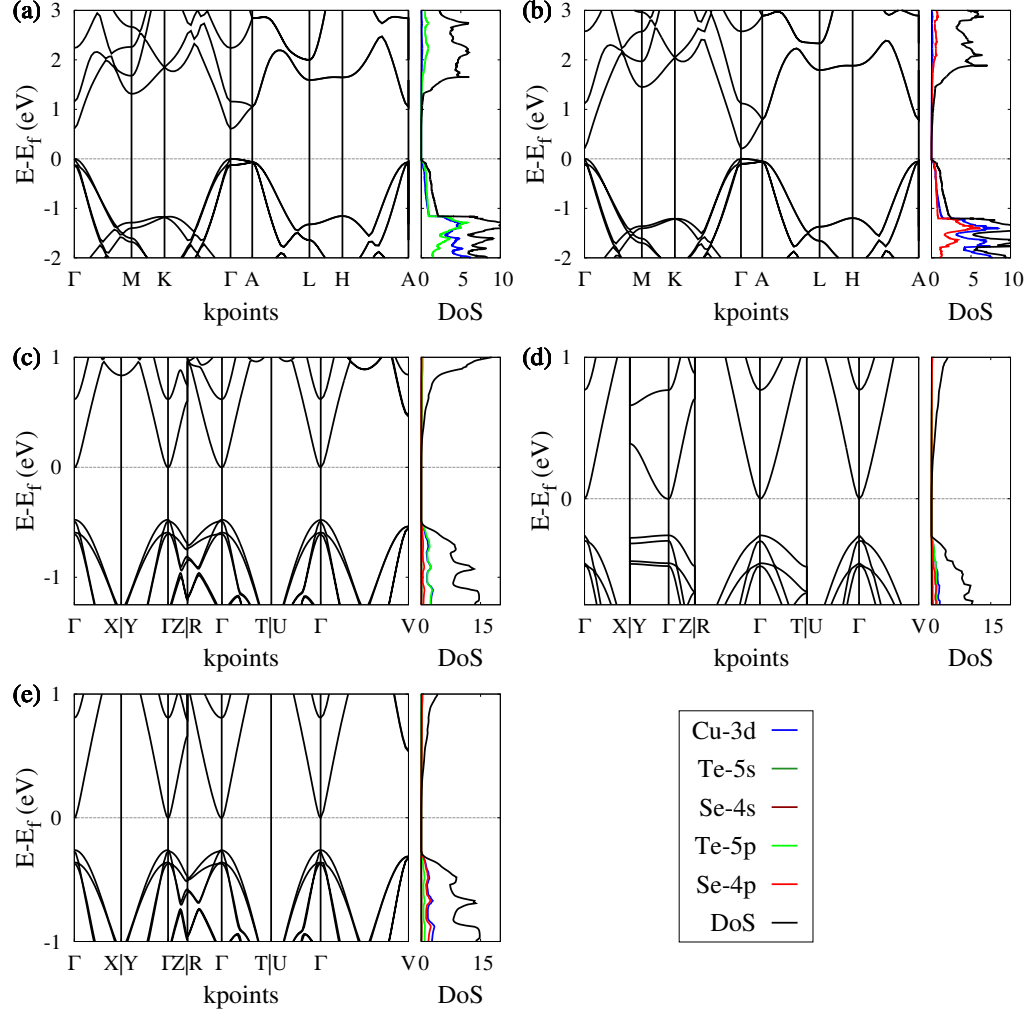

Figure S2: Plots of electronic band structure and density of states of  $\text{KCuTe}_{1-x}\text{Se}_x$  at a)  $x = 0$  b)  $x = 1$  c)  $x = 0.25$  d)  $x = 0.5$  e)  $x = 0.75$ .

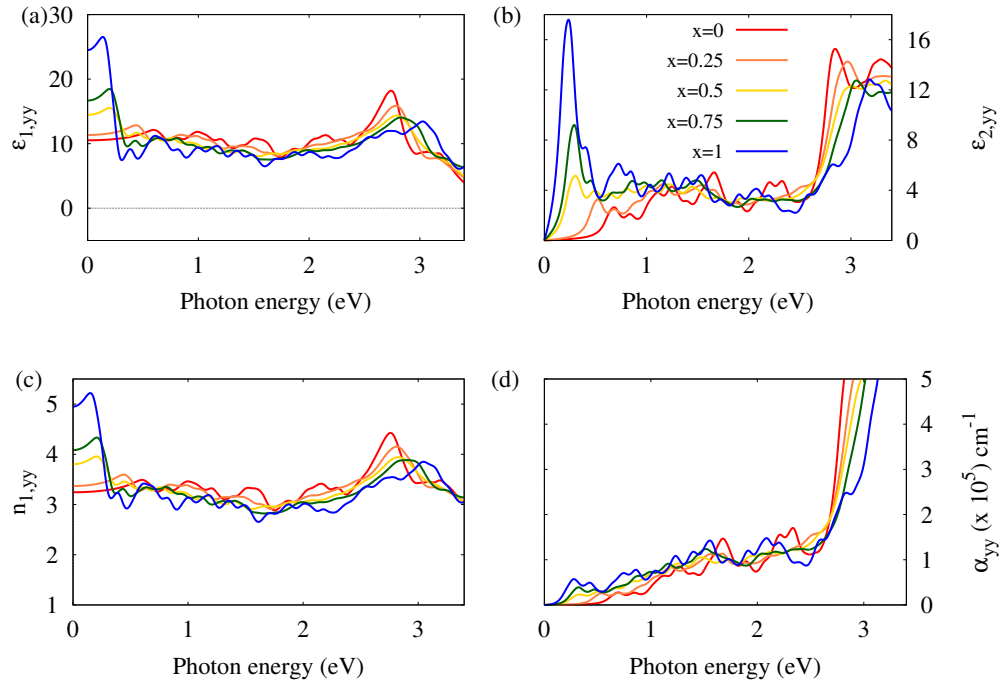

Figure S3: Plots of a) Real part of dielectric constant b) Imaginary part of dielectric constant c) Real part of refractive index and d) Imaginary part of refractive index of  $\text{KCuTe}_{1-x}\text{Se}_x$  at different concentrations for y-polarized light.

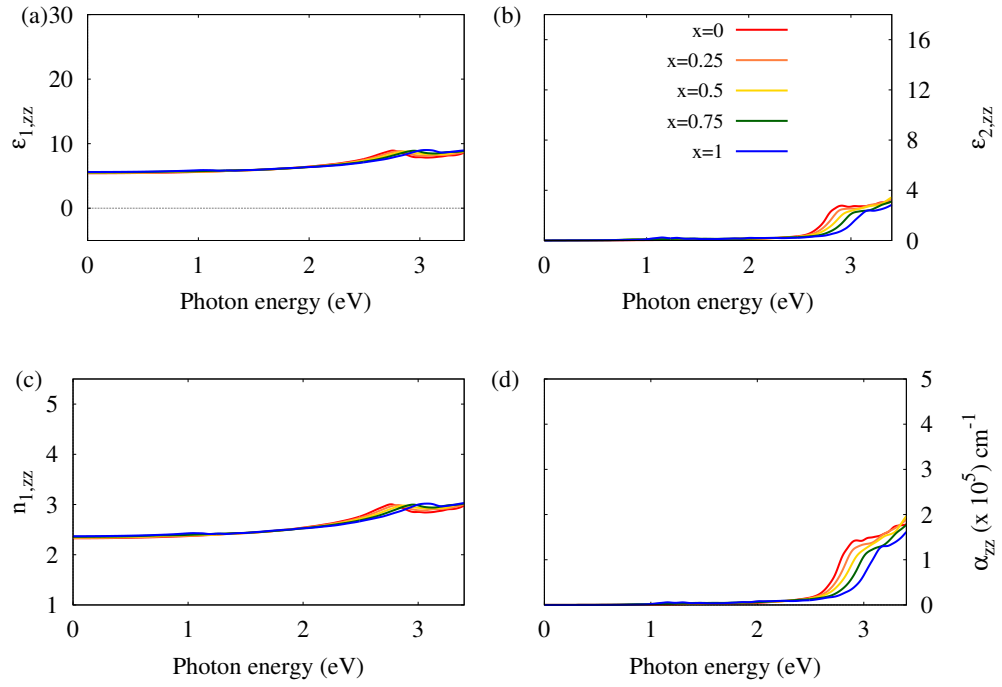

Figure S4: Plots of a) Real part of dielectric constant b) Imaginary part of dielectric constant c) Real part of refractive index and d) Imaginary part of refractive index of  $\text{KCuTe}_{1-x}\text{Se}_x$  at different concentrations for z-polarized light.
